# Supplementary material for: AffectNet+: A Database for Enhancing Facial Expression Recognition with Soft-Labels
Source: arXiv:2410.22506 source file (2024-10-29)
Supplement: Supplementary file 1 [file action_units_correlation.tex]

\begin{table}[b] 
\caption{The correlation between the action units regarding each emotion class.}
\label{tbl:action_units_correlation_supp}
\centering
\small
\resizebox{0.48\textwidth}{!}
{{
\begin{tabular}{lccccccc}
\hline 
\multicolumn{1}{c}{}         & \multicolumn{1}{c}{Happy} & \multicolumn{1}{c}{Sad} & \multicolumn{1}{c}{Surprise} & \multicolumn{1}{c}{Fear} & \multicolumn{1}{c}{Anger} & \multicolumn{1}{c}{Disgust} & \multicolumn{1}{c}{Contempt} \\ \hline

Happy   & \multicolumn{1}{c}{0}     & \multicolumn{1}{c}{1}   & \multicolumn{1}{c}{0}        & \multicolumn{1}{c}{1}    & \multicolumn{1}{c}{1}     & \multicolumn{1}{c}{1}       & \multicolumn{1}{c}{1}        \\ 

Sad   & \multicolumn{1}{c}{1}     & \multicolumn{1}{c}{0}   & \multicolumn{1}{c}{1}        & \multicolumn{1}{c}{2}    & \multicolumn{1}{c}{2}     & \multicolumn{1}{c}{1}       & \multicolumn{1}{c}{0}        \\ 
Surprise & \multicolumn{1}{c}{0}     & \multicolumn{1}{c}{1}   & \multicolumn{1}{c}{0}        & \multicolumn{1}{c}{5}    & \multicolumn{1}{c}{2}     & \multicolumn{1}{c}{1}       & \multicolumn{1}{c}{0}        \\ 
Fear     & \multicolumn{1}{c}{1}     & \multicolumn{1}{c}{2}   & \multicolumn{1}{c}{5}        & \multicolumn{1}{c}{0}    & \multicolumn{1}{c}{4}     & \multicolumn{1}{c}{2}       & \multicolumn{1}{c}{0}        \\ 
Anger    & \multicolumn{1}{c}{1}     & \multicolumn{1}{c}{2}   & \multicolumn{1}{c}{2}        & \multicolumn{1}{c}{4}    & \multicolumn{1}{c}{0}     & \multicolumn{1}{c}{4}       & \multicolumn{1}{c}{0}        \\ 
Disgust  & \multicolumn{1}{c}{1}     & \multicolumn{1}{c}{1}   & \multicolumn{1}{c}{1}        & \multicolumn{1}{c}{2}    & \multicolumn{1}{c}{4}     & \multicolumn{1}{c}{0}       & \multicolumn{1}{c}{0}        \\
Contempt & \multicolumn{1}{c}{1}     & \multicolumn{1}{c}{0}   & \multicolumn{1}{c}{0}        & \multicolumn{1}{c}{0}    & \multicolumn{1}{c}{0}     & \multicolumn{1}{c}{0}       & \multicolumn{1}{c}{0}        \\ \hline
\end{tabular}
}}
\end{table}
