# Supplementary material for: AffectNet+: A Database for Enhancing Facial Expression Recognition with Soft-Labels
Source: arXiv:2410.22506 source file (2024-10-29)
Supplement: Supplementary file 2 [file action_units_for_exp.tex]

\begin{table}[b] 
\caption{Action units for different expressions \cite{martinez2017automatic}.}
\label{tbl:action_units_exp_supp}
\centering
\small
\resizebox{0.3\textwidth}{!}
{{
\begin{tabular}{lccccccc}
\hline
\multicolumn{1}{l}{}           & \multicolumn{7}{c}{Action Units}                                                                                                                                                                              \\ \hline
\multicolumn{1}{l}{Happy}      & \multicolumn{7}{l}{6, 12, 25}                                                                                                                                                                                 \\ 
\multicolumn{1}{l}{Sad}        & \multicolumn{7}{l}{1, 4, 6, 11, 15, 17}                                                                                                                                                                       \\ 
\multicolumn{1}{l}{Surprise}   & \multicolumn{7}{l}{1, 2, 5, 26, 27}                                                                                                                                                                           \\
\multicolumn{1}{l}{Fear}       & \multicolumn{7}{l}{1, 2, 4, 5, 20, 25, 26, 27}                                                                                                                                                                 \\
\multicolumn{1}{l}{Anger}      & \multicolumn{7}{l}{4, 5, 7, 10, 17, 22, 23, 24, 25, 26}                                                                                                                                                       \\ 
\multicolumn{1}{l}{Disgust}    & \multicolumn{7}{l}{9, 10, 16, 17, 25, 27}                                                                                                                                                                      \\ 
\multicolumn{1}{l}{Contempt}   & \multicolumn{7}{l}{12, 14}    \\                                      \hline
\end{tabular}
}}
\end{table}
