# Supplementary material for: AffectNet+: A Database for Enhancing Facial Expression Recognition with Soft-Labels
Source: arXiv:2410.22506 source file (2024-10-29)
Supplement: Supplementary file 3 [file annotator_dist.tex]

\begin{table}[] 
\caption{The correspondence between the number of annotators and images in the \textit{gold-set}.}
\label{tbl:annotator_dist_supp}
\centering
\small
\resizebox{0.48\textwidth}{!}
{{
\begin{tabular}{lcccc}
\hline
\textbf{\# Annotators} & Two   & Three & Four & Five \\ 
\textbf{\# Images}     & 32378 & 2373  & 997  & 302  \\ \hline
\end{tabular}
}}
\end{table}
