# Supplementary material for: AffectNet+: A Database for Enhancing Facial Expression Recognition with Soft-Labels
Source: arXiv:2410.22506 source file (2024-10-29)
Supplement: Supplementary file 7 [file resnet_hard_label_accuracy.tex]

\begin{table}[t!] 
\caption{Accuracy on different sets of AffectNet+ on ResNet-50\cite{he2016deep}.}
\label{tbl:resnet_hard_label_accuracy_supp}
\centering
\small
\resizebox{0.4\textwidth}{!}
{{
\begin{tabular}{lcccc}
\hline
        & All   & Normal & Challenging & Hard  \\ \hline 
Acc (\%)    & 52.06 & 85.86  & 51.62       & 34.34 \\
$\overline{Acc}$ (\%) & 52.04 & 78.13  & 52.38       & 39.15 \\ \hline 
\end{tabular}}}
\end{table}
