# Supplementary material for: AffectNet+: A Database for Enhancing Facial Expression Recognition with Soft-Labels
Source: arXiv:2410.22506 source file (2024-10-29)
Supplement: Supplementary file 9 [file resnet_soft_label_error.tex]

\begin{table}[t!] 
\caption{Error on different sets of AffectNet+ on ResNet-50\cite{he2016deep}.}
\label{tbl:resnet_soft_label_error_supp}
\centering
\small
\resizebox{0.35\textwidth}{!}
{{
\begin{tabular}{lcccc}
\hline
                  & All   & Normal & Challenging & Hard  \\ \hline
W-FR (\%)    & 10.85     & 8.00     & 11.90       & 18.66 \\
W-MAE (\%)   & 17.30      & 15.43      & 18.54        & 21.21  \\
% $\text{W-AUC}_{\epsilon}$    & ?    & ?     & ?      & ? \\ 
\hline
\end{tabular}}}
\end{table}
