# Supplementary material for: AffectNet+: A Database for Enhancing Facial Expression Recognition with Soft-Labels
Source: arXiv:2410.22506 source file (2024-10-29)
Supplement: Supplementary file 10 [file resnet_soft_label_error_on_expression.tex]

\begin{table}[t!] 
\caption{Failure rate, mean average error, and AUC on soft labels, based on the ResNet-50\cite{he2016deep} model, on different expressions.}
\label{tbl:resnet_soft_label_error_on_expression_supp}
\centering
\small
\resizebox{0.48\textwidth}{!}
{{
\begin{tabular}{llcccc}
\hline
                          &     & All   & Normal & Challenging & Hard  \\  \hline
\multirow{3}{*}{Neutral}  & W-FR  & 9.60  & 5.54   & 21.11       & 17.91 \\
                          & W-MAE & 17.46 & 15.29  & 22.60       & 23.09 \\
                          % & $\text{W-AUC}_{\epsilon}$  &       &        &             &       \\ 
                          \hdashline
\multirow{3}{*}{Happy}    & W-FR  & 3.60  & 2.24   & 12.50       & 19.05 \\
                          & w-MAE & 12.59 & 11.27  & 18.24       & 22.84 \\
                          % & $\text{W-AUC}_{\epsilon}$  &       &        &             &       \\ 
                          \hdashline
\multirow{3}{*}{Sad}      & W-FR  & 11.60 & 8.48   & 10.48       & 19.20 \\
                          & W-MAE & 18.14 & 16.85  & 17.07       & 20.39 \\
                          % & $\text{W-AUC}_{\epsilon}$  &       &        &             &       \\ 
                          \hdashline
\multirow{3}{*}{Surprise} & W-FR  & 12.60 & 13.51  & 13.64       & 18.18 \\
                          & W-MAE & 18.25 & 17.60  & 18.43       & 20.43 \\
                          % & $\text{W-AUC}_{\epsilon}$  &       &        &             &       \\ 
                          \hdashline
\multirow{3}{*}{Fear}     & W-FR  & 17.80 & 20.14  & 11.70       & 25.13 \\
                          & W-MAE & 19.42 & 18.71  & 18.92       & 22.43 \\
                          % & $\text{W-AUC}_{\epsilon}$  &       &        &             &       \\ 
                          \hdashline
\multirow{3}{*}{Disgust}  & W-FR  & 12.00 & 16.26  & 15.00       & 19.75 \\
                          & W-MAE & 18.14 & 18.18  & 19.55       & 21.86 \\
                          % & $\text{W-AUC}_{\epsilon}$  &       &        &             &       \\ 
                          \hdashline
\multirow{3}{*}{Anger}    & W-FR  & 11.20 & 8.41   & 12.35       & 12.07 \\
                          & W-MAE & 17.80 & 17.12  & 19.29       & 19.39 \\
                          % & $\text{W-AUC}_{\epsilon}$  &       &        &             &       \\ 
                          \hdashline
\multirow{3}{*}{Contempt} & W-FR  & 8.40  & 3.92   & 6.80        & 14.29 \\
                          & W-MAE & 16.55 & 19.56  & 17.12       & 20.84 \\
                          % & $\text{W-AUC}_{\epsilon}$  &       &        &             &       \\ 
                          \hline
\end{tabular}
}}
\end{table}
